# Supplementary material for: Magnon-polarons in van der Waals antiferromagnet FePS3
Source: arXiv:2108.10945 source file (2021-10-19)
Supplement: Supplementary file 1 [file Supplement.pdf]

# Supplementary Materials for

## Magnon-polarons in van der Waals antiferromagnet $FePS_3$

D. Vaclavkova[1†], M. Palit[2†], J. Wyzula[1], S. Ghosh[2], A. Delhomme[1], S. Maity[2], P. Kapuściński[1,3], A. Ghosh[2], M. Veis[1,4], M. Grzeszczyk[1,5], C. Faugeras[1], M. Orlita[1], S. Datta[2]*, M. Potemski[1,5]**

[1]Laboratoire National des Champs Magnétiques Intenses, CNRS-Univ. Grenoble Alpes-UPS-INSA-EFML, 25 Av. Des Martyrs, 38042 Grenoble, France.

[2]School of Physical Sciences, Indian Association for the Cultivation of Science, 2A & B Raja S. C. Mullick Road, Jadavpur, Kolkata – 700032, India.

[3]Department of Experimental Physics, Wrocław University of Technology, Wybrzeże Wyspiańskiego 27, 50-370 Wrocław, Poland.

[4]Institute of Physics, Charles University, Ke Karlovu 5, Prague, 121 16, Czech Republic.

[5]Institute of Experimental Physics, Faculty of Physics, University of Warsaw, ul. Pasteura 5, 02-093 Warszawa, Poland.

*Corresponding author: subhanano@gmail.com
**Corresponding author: marek.potemski@lncmi.cnrs.fr

†These authors contributed equally to this work.

**This PDF file includes:**

**Supplementary Text**

**Figs. S1 to S3**

## Supplementary Text

*Extraction of resonance energies from the magneto-infrared spectra*: As discussed in the main text, the transmission minima related to $P_1$ and $P_2$ phonons are rather weakly pronounced at low magnetic fields. To extract their positions, we have examined the first derivative of infrared magneto-transmission $dT_B/d\omega$ (Fig. S1a) and searched for the corresponding zero nodes. First, the positions of $P_1$ and $P_2$ modes were identified in the high-field part of the data, where both modes exhibit rather pronounced shifts with the applied magnetic field. Then, the positions were traced, step by step, down to zero magnetic field (green dots in Fig. S1a). The deduced energies of $P_1$ and $P_2$ phonons at $B=0$ were then cross-checked using the zero-field infrared transmission spectrum measured with a higher spectral resolution (0.25 $cm^{-1}$), see Fig. S1b.

**Fig. S1.**

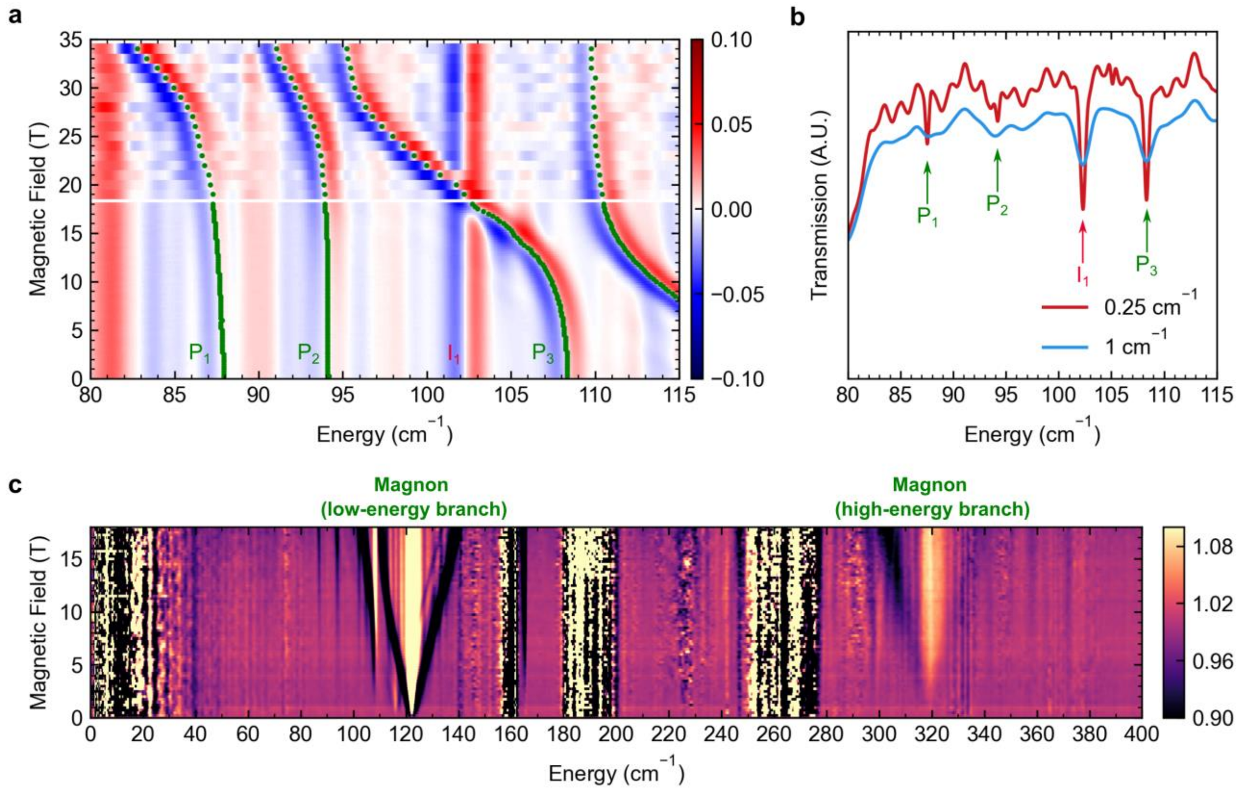


*Fig.* ***S1a****: False-color plot of the first derivative of infrared magneto-transmission, $dT_B/d\omega$, that was measured on bulk $FePS_3$ using the spectral resolution of 1 $cm^{-1}$. The horizontal white line at B = 18 T separates the low- and high-field parts of the data collected using a superconducting and resistive coil, respectively. Fig.* ***S1b****. Raw (= not normalized by reference) infrared transmission spectra of $FePS_3$ measured using the spectral resolution of 0.25 and 1 $cm^{-1}$. The green arrows indicate the positions of $P_1$, $P_2$ and $P_3$ phonon modes. The $I_1$ phonon, marked by red arrow, does not couple with magnon modes and is only visible in transmission measurement (not Raman active). Fig.* ***S1c****: False-colour plot of the relative magneto-transmission, ($T_B/T_0$), measured at low temperatures (T=2.2K) on $FePS_3$. The description indicates the positions of two magnon modes (at ~122 and 318 $cm^{-1}$) with characteristic antiferromagnetic-resonance-like splitting that appears under externally applied magnetic fields.*

**Fig. S2.**

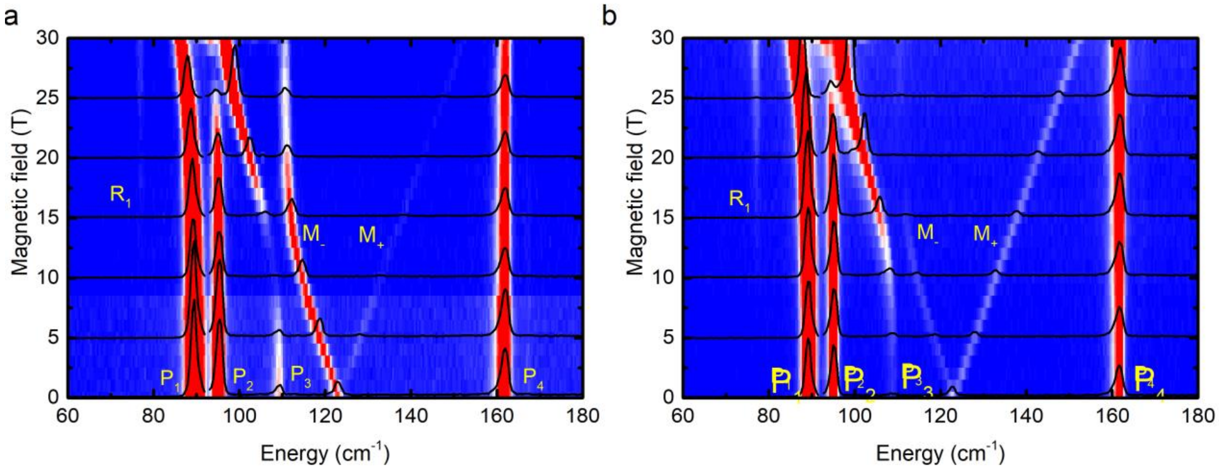


*Fig. S2a: False-color map of magneto Raman scattering response of the $FePS_3$ antiferromagnet, measured at low temperatures of 4.2 K in the configuration of crossed ($\sigma^+/\sigma^-$) circularly polarized beams of the excitation/scattered light with an applied magnetic field oriented perpendicular to the plane of the layers, together with a few selected characteristic spectra. Identical data have been obtained when inverting the polarization scheme to $\sigma^-/\sigma^+$ excitation/scattered beams. Fig. S2b: False-color map of magneto Raman scattering response of the $FePS_3$ antiferromagnet, measured at low temperatures of 4.2 K in the configuration when both the excitation and scattered light are set to have the same ($\sigma^+$) helicity with an applied magnetic field oriented perpendicular to the plane of the layers, together with a few selected characteristic spectra. Identical spectra are measured in case of the excitation and scattered light with the same $\sigma^-$ helicity.*

**Fig. S3**

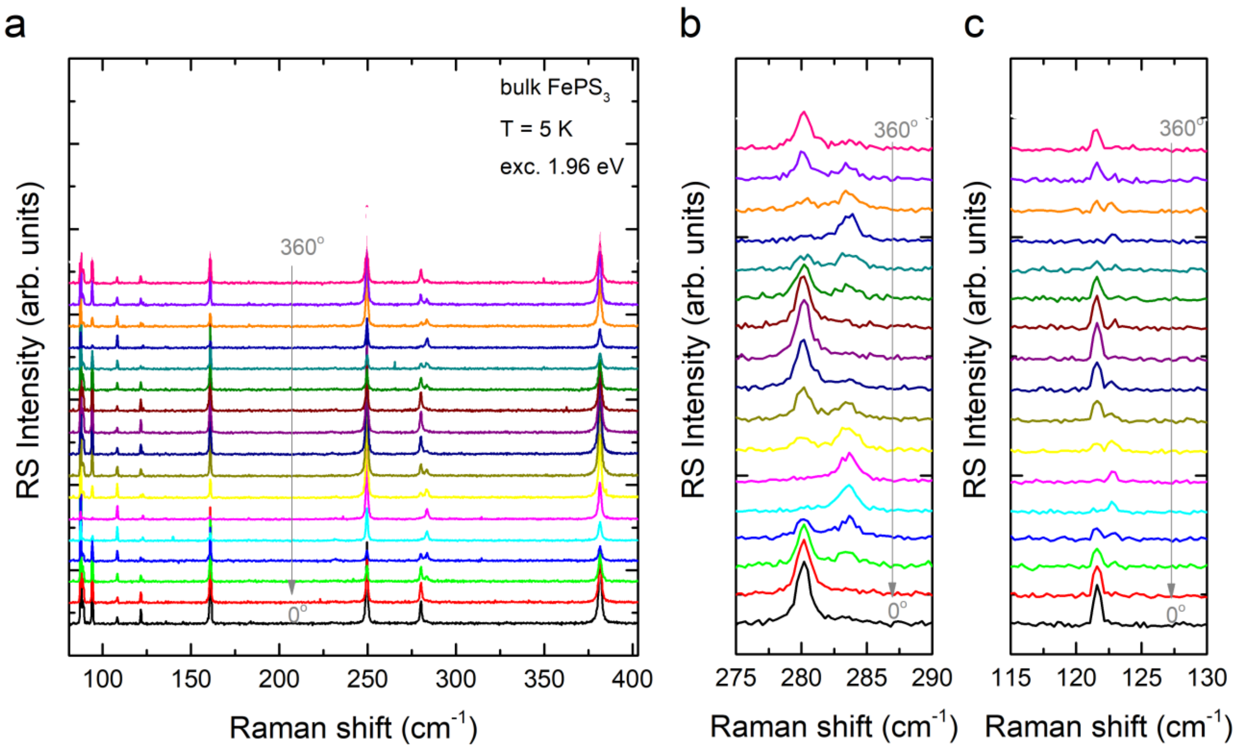


*Fig. S3: Low temperature (4.2 K) Raman scattering spectra of the $FePS_3$ antiferromagnet as a function of the angle between the directions of linear polarisation of the excited and scattered light. The spectra measured in a wide spectral range are shown in (a). The response due to $F_3$ –phonon and M-magnon features are amplified, correspondingly, in (b) and (c). Note that M magnon and $F_3$ phonon doublet components show identical selection rules.*
